# Supplementary material for: Learning How to Walk: Warm-starting Optimal Control Solver with Memory of Motion
Source: arXiv:2001.11751 source file (2020-02-28)
Supplement: Supplementary file 1 [file suplementary.tex]

\section{Supplementary Materials}
\label{sec:supplement}

\subsection{Bayesian Gaussian Mixture Regression (BGMR)}
As discussed in the main text, given the training dataset $\{\bm{X},\bm{Y}\}$ GMR constructs the joint probability of $(\bm{x},\bm{y})$ as a mixture of Gaussians,
\begin{equation}
p(\bm{x},\bm{y}) = \sum_{k=1}^K \pi_k \, \mathcal{N}(\bm{\mu}_k,\bm{\Sigma}_k),
\end{equation}	
where $\pi_k$, $\bm{\mu}_k$, and $\bm{\Sigma}_k$ are the $k$-th component's mixing coefficient, mean, and covariance, respectively. Let $\bm{\theta} = \{\pi_k,\bm{\mu}_k, \bm{\Sigma}_k\}_{k=1}^K$, denoting the GMR parameters to be determined from the data. 

We can decompose $\bm{\mu}_k$ and $\bm{\Sigma}_k$ according to $\bm{x}$ and $\bm{y}$ as
\begin{equation}
\bm{\mu}_k = \begin{pmatrix} \bm{\mu}_{k,x} \\ \bm{\mu}_{k,y} \end{pmatrix} \quad \text{and} \quad \bm{\Sigma}_k = 
\begin{pmatrix}
\bm{\Sigma}_{k,xx} & \bm{\Sigma}_{k,xy} \\
\bm{\Sigma}_{k,yx} & \bm{\Sigma}_{k,yy}
\end{pmatrix}.
\end{equation}
Given a query $\bm{x}^*$, the predictive distribution of $\bm{y}$ can then computed by conditioning on $\bm{x}^*$, 
\begin{equation}
p(\bm{y}|~\bm{x}^*,\bm{\theta}) = \sum_{k=1}^K p(k|~\bm{x}^*,\bm{\theta}) \, p(\bm{y}|~k,\bm{x}^*,\bm{\theta}), 
\label{eq:gmr_pred_sup}
\end{equation}
where $p(k|~\bm{x}^*,\bm{\theta})$ is the probability of $\bm{x}^*$ belonging to the $k$-th component, 
\begin{equation}
p(k|~\bm{x}^*,\bm{\theta}) = \frac{\pi_k \, \mathcal{N}(\bm{x}^* |~ \bm{\mu}_{k,x}, \bm{\Sigma}_{k,xx})}{\sum_{i=1}^{K} \pi_i \, \mathcal{N}(\bm{x}^* |~ \bm{\mu}_{i,x}, \bm{\Sigma}_{i,xx}) },
\label{eq:prob_k}
\end{equation}
and $p(\bm{y}|~k,\bm{x}^*,\bm{\theta}$) is the predictive distribution of $\bm{y}$ according to the $k$-th component, 
\begin{equation}
p(\bm{y}|~k,\bm{x}^*,\bm{\theta}) = \mathcal{N}\Big(\bm{\mu}_{k,y} + \bm{\Sigma}_{k,yx} {\bm{\Sigma}^{-1}_{k,xx}}(\bm{x}^* - \bm{\mu}_{k,x}), \; \bm{\Sigma}_{k,yy} - \bm{\Sigma}_{k,yx} {\bm{\Sigma}^{-1}_{k,xx}} \bm{\Sigma}_{k,xy}\Big),
\label{eq:pred_k}
\end{equation}
which is a Gaussian distribution with the mean being linear in $\bm{x}^*$. The resulting predictive distribution \eqref{eq:gmr_pred_sup} is then a mixture of Gaussians. 

In GMR, $\bm{\theta}$ is usually estimated from the dataset $\{\bm{X},\bm{Y}\}$ by using Expectation-Minimization method that outputs a single value for $\bm{\theta}$, and the prediction is computed using this value. Instead, Bayesian GMR (BGMR) puts priors to the parameter $\bm{\theta}$, and given the dataset $\{\bm{X},\bm{Y}\}$, it computes the posterior distribution $p(\bm{\theta} |~\bm{X},\bm{Y})$. Hence, when we do prediction we have to integrate over the posterior distribution of $\bm{\theta}$, 
\begin{equation}
p(\bm{y}~|~\bm{x}^*, \bm{X},\bm{Y} ) = \int_{\bm{\theta}}^{} p(\bm{y}~|~\bm{x}^*, \bm{\theta}) \, p(\bm{\theta} ~|~ \bm{X},\bm{Y}) \, d\bm{\theta}. 
\label{eq:integrate_post}
\end{equation}
The resulting predictive distribution is then a mixture of multivariate t-distributions, 
\begin{equation}
p(\bm{y}~|~\bm{x}^*, \bm{X},\bm{Y}) = \sum_{k=1}^K p(k~|~\bm{x}^*, \bm{X},\bm{Y}) \, p(\bm{y}~|~k,\bm{x}^*,\bm{X},\bm{Y}), 
\label{eq:bgmr_pred_sup}
\end{equation}
where $p(k\,|\,\bm{x}^*, \bm{X},\bm{Y})$ is the probability of $\bm{x}^*$ belonging to the $k$-th component and $p(\bm{y}~|~k,\bm{x}^*,\bm{X},\bm{Y})$ is the predictive distribution of $\bm{y}$ according to the $k$-th component. These are calculated using the formula similar to \eqref{eq:prob_k} and \eqref{eq:pred_k}, but the Gaussian distributions are replaced by t-distributions. $p(\bm{y}~|~k,\bm{x}^*,\bm{X},\bm{Y})$ is a t-distribution (whose mean is also linear w.r.t.~$\bm{x}^*$) instead of a Gaussian distribution as in \eqref{eq:pred_k}, due to the integration over the posterior distribution in \eqref{eq:integrate_post}. 

%, 
%\begin{equation}
%p(k~|\bm{x}^*,\bm{\theta}) = \frac{\pi_k \mathcal{N}(\bm{x}^* ~| \bm{\mu}_{k,x}, \bm{\Sigma}_{k,xx})}{\sum_{i}^{K} \pi_i \mathcal{N}(\bm{x}^* ~| \bm{\mu}_{i,x}, \bm{\Sigma}_{i,xx}) }
%\end{equation}

%\begin{equation}
%p(\bm{y}^*~|k,\bm{x}^*,\bm{\theta}) = \mathcal{N}(\bm{\mu}_{k,y} + \bm{\Sigma}_{k,yx} {\bm{\Sigma}_{k,xx}}^{-1}(\bm{x}^* - \bm{\mu}_{k,x}), \bm{\Sigma}_{k,yy} - \bm{\Sigma}_{k,yx} {\bm{\Sigma}_{k,xx}}^{-1} \bm{\Sigma}_{k,xy}),
%\end{equation}

Note that the predictive distribution of GMR \eqref{eq:gmr_pred_sup} and BGMR \eqref{eq:bgmr_pred_sup} are very similar, but \eqref{eq:gmr_pred_sup} is a mixture of Gaussians whereas \eqref{eq:bgmr_pred_sup} is a mixture of t-distributions. Both can be seen as a mixture of linear regressions, since the mean prediction according to each $k$-th component \eqref{eq:pred_k} is linear in $\bm{x^*}$. 

The advantage of having a Bayesian version of GMR is the following:
\begin{itemize}
\item When the dimension of $\bm{x}$ and $\bm{y}$ is high, the number of parameters to be estimated in $\bm{\theta}$ is large and the estimation of $\bm{\theta}$ in GMR is prone to overfitting, unless the number of training data is very large. Putting the priors to $\bm{\theta}$ in BGMR helps mitigating the overfitting and makes it possible to learn with fewer number of datapoints.
\item By putting Dirichlet Process prior to the parameters $\pi_k$, the number of components $K$ can be determined automatically. 
\end{itemize}

To illustrate how BGMR can handle multimodal output, we show an illustrative example in Figure \ref{fig:toy_example}, which depicts a mapping $y = f(x)$ that is discontinuous at $x$ = 4 and $x$ = 6, and has two modes at $0 < x < 4$. The data points corresponding to $(x,y)$ are shown in black. First, BGMR fits a mixture of Gaussians to ($x,y$), shown as red ellipses in Figure \ref{fig:toy_example}a. We can see that the Gaussians fit well each mode and each side of discontinuity. 

Given a query point $x^*$, the predictive distribution of $y^*$ is a mixture of t-distributions given by \eqref{eq:bgmr_pred_sup}. Figure \ref{fig:toy_example}b shows an example of $p(y~|x)$ for $x = 0.8$. We can see that there are two peaks corresponding to the two modes of the mapping $f$ (i.e., $y$ = 25.2 and $y$ = 46.7), having roughly the same probability ($0.5$). 

Figure \ref{fig:toy_example}c shows the BGMR predictions over the range of $x$, by taking the mean of the components with the highest and the second-highest probability in \eqref{eq:bgmr_pred_sup}. We see that it predicts both modes very well, and it still performs well at discontinuous region (i.e., it does not average the both sides of discontinuity).

\begin{figure}[t!]
\centering
\subfloat[][]{\includegraphics[width=0.3\columnwidth]{multi_modal_function}\label{fig:toy_example_a}}
\subfloat[][]{\includegraphics[width=0.3\columnwidth]{prob_y}\label{fig:toy_example_b}}
\subfloat[][]{\includegraphics[width=0.3\columnwidth]{bgmr_prediction}\label{fig:toy_example_3}}
\caption{
An example of multimodal and discontinuous mapping $f: x \rightarrow y$. BGMR fits a mixture of Gaussians to the joint data of $\bm{x}$ and $\bm{y}$ (a), resulting in a mixture of t-distributions as the predictive distribution of $y$ given $x^* = 0.8$ (b). By taking the means of the highest and second highest component of the mixture, BGMR approximates the mapping very well (c).}
\label{fig:toy_example}
\end{figure}

%This is especially important for BGMR, since it needs to estimate the covariance matrix $\bm{\Sigma}_k$ which grows quadratically as the number of dimensions. 

%	- Discuss the storage and computational complexity (training and prediction)

% Experiment

%About TrajOpt
%TrajOpt applies sequential convex optimization to solve the motion planning problem. The collision avoidance in TrajOpt is implemented as soft constraint with an outer loop that increases the penalty weight if the constraints are not satisfied by the current solution. TrajOpt has two collision costs: discrete and continous. The discrete collision cost is based on the signed distance between the robot's links and the obstacles at the time step $t$, while the continuous collision cost consider the volume swept by the links between the time steps. The continuous collision cost enables TrajOpt to plan with much fewer time steps as compared to the other methods. However, it does not check self-collisions. We therefore use both costs in all our experiments.  
%
%In Section 4.1, the initial pose 
%
%
%In Section 4.2, the initial joint configuration is depicted in Figure ***, while the goal configuration is randomly sampled while 
%\td{The initial and goal configurations have both arms outside and inside the shelf, respectively}. 
%\td{In both configurations the hands are inside the shelf.} 
%
%while the orientations and the initial joint configurations are kept fix.

% Algorithm
